# Supplementary material for: Efficiently Checking Actual Causality with SAT Solving
Source: arXiv:1904.13101 source file (2019-04-30)
Supplement: Supplementary file 1 [file appendix.tex]

\section{Appendix: Proofs}\label{sec:ac3_proof}
Before presenting the proof, we define the term \textit{non-minimal cause}.
\begin{definition} \label{def:non-minmal} \textbf{Non-minimal Cause}\
	is a tentative cause $\vec{X_{(n)}} = \vec{x}_{(n)}$ that contains at least one element $X_n$ that satisfies one of the following conditions
	\begin{itemize}
		\item\textbf{NMC1.} Removing $X_n$ from $\vec{X_{(n)}}$ and adding it to $\vec{W}$, results in AC2 holding for the remaining tentative cause $\vec{X}_{(n-1)}$, i.e., $(M,\vec{u})\models \bigl[\vec{X}_{(n-1)}\leftarrow \vec{x}_{(n-1)}',X_n\leftarrow x_n,\vec{W}\leftarrow\vec{w}\bigr]\neg\varphi$
		\item \textbf{NMC2.}  AC2 holds for $\vec{X}_{(n-1)}$ regardless of $X_n$, i.e., $X_n \in \vec{W} \vee X_n \not\in \vec{W}$
		\item \textbf{NMC3.}  AC2 holds for $\vec{X}_{(n-1)}$ only if $X_n \not\in \vec{W}$, i.e., $(M,\vec{u})\models \bigl[\vec{X}_{(n-1)}\leftarrow \vec{x}_{(n-1)}',\vec{W}\leftarrow\vec{w}\bigr]\neg\varphi$
	\end{itemize}
\end{definition}
It is worth noting that a non-minimal cause $\vec{X}$ may contain multiple elements that satisfy different conditions. Informally, the first condition covers the case where part of the non-minimal cause should actually be considered in $\vec{W}$. In this case, AC2 does not even hold for the non-minimal cause. The second condition deals with irrelevant variables, i.e., those that don't affect the cause relation to the effect. The third condition targets the case of relevant variables that are affected by the cause but not necessary for it to be a cause. For a non-minimal cause containing elements that satisfy condition two and three, AC2 holds. 
\repeattheorem{ac3}

\begin{proof}

	\begin{proofpart}
		If the cause is a non-minimal cause, then Algorithm.\ref{algorithm:fulfillsac3_sat} returns 0 	
	\end{proofpart}
	\noindent For the algorithm to return 0, $G$ must be satisfiable. So we prove this part by showing that if any of the conditions in Def.\ref{def:non-minmal} hold then $G$ is satisfiable and the algorithm returns 0.%. We treat the two conditions \textit{NMC1 and NMC2} as the same.
	\begin{enumerate}
		\item Recall $G := \neg\varphi \wedge \bigwedge_{i=1\ldots\ell} f(U_i=u_i)\wedge\bigwedge_{i=1\ldots m, \not\exists j\bullet X_j=V_i} \left(V_i \leftrightarrow F_{V_i} \lor f(V_i=v_i)\right)	\wedge\bigwedge_{i=1\ldots\ell} (X_i\lor\neg X_i)$. Let us rewrite the formula to abstract the first part as, $G:= G_{base}\wedge\bigwedge_{i=1\ldots n}( X_i\lor\neg X_i)$.  
		\item  Note how  $\vec{X_{(n)}}$ is added to $G$ as $ (X_1 \vee \neg X_1)\wedge(X_2 \vee \neg X_2)\dots (X_n \vee \neg X_n)$. Re-write this big conjunction to its equivalent disjunctive normal from (DNF) i.e., $ (\neg X_1 \wedge \neg X_2 \dots \wedge \neg X_n) \lor(\neg X_1 \wedge \neg X_2 \dots \wedge X_n)\dots\lor(X_1 \wedge X_2 \dots \wedge X_n)$. Assume wlog
		that all the actual values of $\vec{X_{(n)}}$ were \textit{true}, hence to check them in AC2 we need to have their values negated, i.e., $\neg X_i$. Looking at the DNF, we have $2^n$ clauses that list all the possible cases of negating or fixing the elements in $\vec{X}$. Then, we partition $G$ according to the clauses, i.e, $G:=G_1 \lor G_1\dots G_{2^n}$, where $G_1:=G_{base}\wedge (\neg X_1 \wedge \neg X_2 \dots \wedge \neg X_n)$. In the case of the clause where all variables $\vec{X_{(n)}}$ are negated, the corresponding $G$, i.e., $G_1$, is exactly formula $F$ from Algorithm.\ref{algorithm:fulfillsac2_sat}.
		\item Each $G_i$, other than $G_1$, fixes some group of elements to their original evaluation ($X_i$) and negates some, possibly none ($G_{2^n}$), other elements ($\neg X_i$). Clearly, $G_i$ is an $F$ formula (from Algorithm.\ref{algorithm:fulfillsac2_sat}) for all the negated variables, in a clause, as $\vec{X}$ but with a special fixed variables that are added to $\vec{W}$. Hence, a $G_i$ is a check of AC2 for a specific subset of the causes given that the other part (fixed) of the cause is in $\vec{W}$. This exactly is the case of the first two conditions in Def.\ref{def:non-minmal}, i.e, AC2 holds after transferring some elements $\vec{X^*}$ from $\vec{X}$ to $\vec{W}$.  $\vec{X^*}$ is guaranteed to be expressed in one of the $2^n$ clauses, and hence, by a specific $G_k$. According to Theorem.\ref{theorem:F}, such a $G_k$ is satisfiable since AC2 holds. Then, for a non-minimal cause based on condition one or two of Def.\ref{def:non-minmal}, $G$ is satisfiable since $G_k$ is satisfiable. In the algorithm, it is easy to see that $\forall i \in \vec{X^*} v_i' = v_i$ since they should be in $\vec{W}$, and hence the algorithm returns 0.     
		%\If{$|\bigl\{j\in\{1,..,\ell\}|\exists i\bullet V_i=X_j\land v_i'\not=v_i$ \WRP$\land v_i'\not= [\overrightarrow{V} \leftarrow \vec{v}'] F_{X_i}\bigr\}| < \ell$}
		\item Similarly, for the third case, i.e., the non-minimal part should not be in $\vec{W}$. In this case, AC2 holds for the non-minimal cause, i.e, $F$ and $G_1$ are satisfiable and then $G$ is also satisfiable. Since the non minimal parts in this case are not in $\vec{W}$ or $\vec{X}$, then they follow their equations in the model, and hence $ \exists i \bullet v_i'=[\overrightarrow{V} \leftarrow \vec{v}'] F_{X_i}$, which results in 0 returned by the algorithm. 
	\end{enumerate}
	
	\begin{proofpart}
		If Algorithm\ref{algorithm:fulfillsac3_sat} returns 0, then the cause is a non-minimal cause 
	\end{proofpart}
	
	\noindent The algorithm would return 0 only if $G$ was satisfiable, which  is when $\vec{X}$ only, a subset of $\vec{X}$ only, or both fulfills AC2.  Now we only have to show that if $\vec{X}$ only fulfills AC2, i.e., $\vec{X}$ is a minimal cause, the algorithm does not return 0. By lemma.\ref{lemma:negation}, a cause should have all its elements negated. Hence the first conjunct in line \ref{alg:line:fulfillsac3_sat:new_cause} of Algorithm.\ref{algorithm:fulfillsac3_sat} will be \textit{true} for each element. If the second conjunct in the same line ($v_i'\not=[\overrightarrow{V} \leftarrow \vec{v}'] F_{X_i}$) evaluates to \textit{false} for any element then, this is not a minimal cause. Hence, for a minimal cause the two conjuncts will evaluate to true for all the elements in $\vec{X}$, and then a 0 is never returned for such a case. 
\end{proof}

%If G is not satisfiable, then \vec{X} is  minimal in the sense that no subset of it fulfills AC2, however in that case x also doesn’t.
